# Supplementary material for: Casablanca: Data and Models for Multidialectal Arabic Speech Recognition
Source: arXiv:2410.04527 source file (2024-10-06)
Supplement: Supplementary file 1 [file Related_work_SER.tex]

\subsection{Speech Emotion Recognition}
\label{app:ser}
Speech Emotion Recognition (SER) represents a critical challenge in human-to-machine interaction. It entails recognizing and interpreting emotions from spoken languages, allowing machines to understand (and potentially produce) human emotions. There are two main paradigms for emotion recognition: Discrete emotions \cite{EkmanEmotions} with specific categories to choose from (sad, happy, etc.) and emotional dimensions \cite{EmotionDimensions}, where emotions are measured on three continuous scales: valence (the pleasantness of a stimulus), arousal (the intensity of emotion provoked by a stimulus), and dominance (the degree of control exerted by a stimulus). In both paradigms, the lack of data is the main barrier to creating reliable and robust SER systems. In this text, we will focus on Discrete Emotions. Emotional Databases are categorized into three primary types: Acted, elicited, and natural. Acted databases \cite{ActedEmotions} feature recordings by trained actors portraying specific emotions, offering control and accessibility for adjustments, but are highly dependent on speaker skills. Elicited databases \cite{ElicitEmotions} involve placing participants in scenarios designed to evoke genuine emotional responses, which proved to be very difficult as it also requires ethical consent. Natural databases (gathered from real-world interactions like podcasts, conversations, and call centers) provide the most authentic data but may face limitations in the range of emotions. English is miles ahead of other languages when it comes to emotional databases because of the early investment and extensive research in English-language speech emotion processing. IEMOCAP \cite{IEMOCAP} is the most used benchmark dataset for discrete speech emotion recognition, consisting of over 12 hours of acted recordings (audio + video) by 10 actors (5 females and 5 males), each recording falling into one of nine emotion categories (neutral, happiness, sadness, anger, surprise, fear, disgust, frustration, excited and other).  Another widely used English dataset is MSP-IMPROV \cite{MSPIPROV}, a multimodal (audio and video) resource primarily focused on spontaneous emotions within acted improvisations. It was collected with the goal of creating more natural and complex emotional data for training and evaluating speech emotion recognition (SER) systems. It contains about 18 hours of spontaneous dyadic improvisations with four main labels (Anger, Happiness, Sadness, and Neutral). One of the few completely natural datasets in SER is The CMU-MOSEI (Multimodal Opinion Sentiment and Emotion Intensity) \cite{CMUMOSEI}, With over 23,000 video segments and 65 hours of data it is considered the biggest emotion recognition dataset to date. It is composed of thousands of YouTube videos featuring monologues from a diverse range of speakers covering various topics and providing authentic emotional speech samples in a conversation-like setting.
