# Supplementary material for: Casablanca: Data and Models for Multidialectal Arabic Speech Recognition
Source: arXiv:2410.04527 source file (2024-10-06)
Supplement: Supplementary file 2 [file subdialects.tex]

\subsection{Subdialects}\label{sec:subdialects}
\textbf{Algeria:} with 58 cities and Modern Standard Arabic as an official language. However, most people (75\% to 80\%) speak local Algerian Arabic dialects, collectively known as Daridjah. These dialects came about because of two big waves of Arab influence in the 7th and 11th centuries, mixing Arabic with the local Berber language. Algerian Daridjah is rich and complex, mixing many words from Turkish, French, Italian, and Spanish because of a long history of colonization \cite{bougrine-2017}. People often switch between languages, especially with French. According to \newcite{pereira2011arabic} there are two main types of Algerian Arabic dialects: \textit{\textbf{(1) Pre-Hilali dialects}:} Spoken in certain cities and their surrounding rural areas are ancient and well-established, dating back to the spread of Islam in the 7th century. Cities such as Tlemcen and Constantine are notable for preserving these dialects, while in other regions, Berber languages remained predominant. \textit{\textbf{(2)  Bedouin dialects}:} These came with Arab newcomers in the 11th century. They're divided into four: \textit{(i) Sulaymite}: Similar to Tunisian Bedouin dialects. \textit{(ii) Ma’qilian}: Close to Moroccan Bedouin dialects. \textit{(iii) Hilali}: Has three kinds of nomadic dialects, including one across the Algerian Sahara, one in the Tell region and the Highplains of Constantine, and \textit{(iv) Completely-Bedouin}: Found in Algiers and some coastal cities. This last one is split further into Algiers-Blanks and Sahel-Tell because of some differences.

\textbf{Egypt:} We discern two primary sub-dialects within the Egyptian Arabic dialect: Cairene and Urban Upper Egyptian Arabic. Cairene Arabic, predominantly spoken in the capital, Cairo, in the southern part of the Nile Delta, has achieved widespread popularity, partly due to its significant presence in various forms of mass media, including television series, songs, films, and soap operas \cite{behnstedt2018formation}. It is characterized by orthographic features diverging from Standard Arabic, influencing pronunciation and written expression. A prominent phonetic aspect of Cairene Arabic is the transformation of the \<ق>[q] sound into a glottal stop \<ء>[\textipa{P}], exemplified by the word \<قهوة> (coffee) being pronounced as '\<ʔ>ahwah' and \<قمر> (moon) as '\<ʔ>amar'. The majority of characters in our series predominantly utilize Cairene Arabic. Conversely, the Urban Upper Egyptian Arabic, also known as Saidi, is the other sub-dialect identified in our annotations. The Saidi sub-dialect is characterized by its unique pronunciation and written representation of sounds distinct from other regional varieties \cite{woidich1996rural}. A notable example is the pronunciation of the letter \<ج> [g] as in "gabal" (mountain), which is articulated as an affricate ǧ or dj in Upper Egypt and the eastern Delta regions. This linguistic analysis underscores the rich diversity and complexity inherent in the Arabic language, particularly within its regional dialects and sub-dialects.

\textbf{Jordan:} Within the Jordanian dialect, we distinguish three primary sub-dialects: the Northern Jordanian Dialects, the Urban or Madani dialect, and the Southern Jordanian Dialects. The Northern Jordanian Dialects, found in areas like Irbid and Ajloun, share close ties with southern Syrian dialects, reflecting historical and geographical connections. The Urban or Madani dialect is mainly used in Jordan's urban hubs such as Amman and Aqaba, drawing on a diverse array of linguistic influences from the Levant and beyond \cite{al2007formation}. The Southern Jordanian Dialects, typical in cities like Al-Karak, integrate features of the Northern dialects with Bedouin linguistic elements.

\textbf{Morocco:} For the Moroccan dialect, the annotators identify two main Arabic sub-dialects: the Shamali, predominant in the north and spoken in locales such as Tangier and Tétouan, and the dialects from Casablanca and the Soussi region, the latter being characteristic of the south, including areas like Agadir and Marrakech \cite{francisco2021southern, announi2021moroccan}.

\textbf{Yemen:} In the case of the Yemeni dialect, we pinpointed five sub-dialects. The Sana'ani dialect is widespread in and around the capital, Sana'a; the Hadrami and Ta'izzi dialects are respectively found in the Hadramaut and Taiz regions; the Adeni dialect is common in Aden, and the Tihami or Tihāmiyyah dialect is spoken along the Red Sea coast in the Tihamah region \cite{watson2013definition}.

\textbf{UAE:} Regarding the Emirati dialect, our analysis revealed three sub-dialects corresponding to various regions across the UAE. The Western Coastal dialect is notably prevalent, while the Eastern Coastal dialect, especially from Kalba, appears less frequently. Additionally, the diverse Bedouin dialects are represented, albeit less commonly than the Western Coastal dialect.

\textbf{Palestine:} The Palestinian dialect exhibits two sub-dialects in the annotated series. These sub-dialects are the Urban Madani dialect and the rural Fallahi dialect. The Urban Madani dialect is predominantly used by the inhabitants of major Palestinian cities, reflecting the influence of diverse civilizations and cultures, especially notable in Haifa and Nablus and, to a lesser extent, in Jerusalem, Hebron, Akka, and Nazareth. This dialect distinguishes itself through specific linguistic features, including the conversion of the \<ق>  sound (q) into a glottal stop (\textipa{P}), the replacement of the voiced dental fricative \<ذ> with the sound \<ز> (z), and the practice of code-switching, incorporating terms from various languages, including Turkish and English \cite{palva1984general}. 
In contrast, the Rural Fallahi Dialect, spoken across Palestinian villages, varies depending on geographic location and proximity to linguistic influences from neighboring regions. This dialect also shows unique adaptations in areas close to Hebron, Jaffa, and Gaza, illustrating the diverse linguistic landscape within Palestinian rural communities.

\textbf{Hassaniya:} The Hassaniya dialect, a variant of the Maghrebi Arabic dialects, is predominantly spoken by the Arabic-speaking majority in Mauritania and extends to six additional countries: Morocco, Algeria, Mali, Libya, Senegal, and Niger\footnote{\url{https://en.wikipedia.org/wiki/Hassaniya_Arabic}}. The linguistic practice among Hassaniya speakers prominently features code-switching, a phenomenon influenced by colonial legacies, which manifests distinctively across different regions or countries. For example, the speakers of Hassaniya in Morocco, commonly alternate between Hassaniya and Spanish, reflective of the colonial history of the Al Sakia Al Hamra and Wadi Al Dhahab regions. Conversely, in Mauritania, the linguistic interchange predominantly involves French, Wolof, Fulan, and Zenaga \cite{taine_cheikh_2020}. The data presented in this work is from Mauritanian Hassaniya, so the varieties present are the ones naturally occurring within Mauritania. Our annotators have noticed two major sub-dialects: Sharg and Gibla mainly spoken in the East and South of Mauritania. The variations among these sub-dialects primarily manifest in vocabulary and usage \cite{ALANY+1969+15+19}.

% \textcolor{red}{\small Yemeni (didn't release the dataset): https://link.springer.com/article/10.1007/s13369-023-07670-7} \\

% Series | list of dialects | 

% 100
% Segment ID | sub-dialect 
